# Supplementary material for: Augmented CycleGAN: Learning Many-to-Many Mappings from Unpaired Data
Source: arXiv:1802.10151 source file (2018-06-18)
Supplement: Supplementary file 1 [file 7-old-appendix.tex]

\clearpage
\appendix
\section{Appendix}
\textcolor{red}{\textbf{\emph{Move content of this section in a separate file before submission.}}}

% \subsection{CycleGAN as Two Adversarial Autoencoders}
% \label{sec:adv_ae_cyclegan}
% While the CycleGAN objective imposes intuitive constrains for unsupervised learning of mappings across domains, we show in this section that this objective can be derived using a variational autoencoder framework~\citep{kingma2013auto} and connect it to the adversarial autoencoder model introduced in~\citep{makhzani2015adversarial}.
% % Specifically, we show that CycleGAN is composed of two adversarial autoencoders, where in the first $\A$ is the observations domain and $\B$ is the latent codes domain, and in the second $\B$ is the observation domain while $\A$ is the latent codes domain.

% In a probabilistic terms, CycleGAN estimates the true conditionals using $q_\phi(b | a)$ defined by the forward mapping $F_\phi$, and $p_{\theta}(a | b)$, defined by the backward mapping $G_\theta$. Using these conditionals, we can define the following distributions:
% \begin{eqnarray}
% p_{\theta}(a,b) &= &p_{\theta}(a | b)\pdata(b) \\
% q_\phi(a,b) &= &q_\phi(b | a)\pdata(a) \\
% p_\theta(a) &= &\int p_\theta(a | b) \pdata(b) db \\
% q_\phi(b) &= &\int q_\phi(b | a) \pdata(a) da
% \end{eqnarray}

% Consider an autoencoder in which $\A$ acts as the observation space and $\B$ as the latent space, i.e. $q_\phi(b | a)$ is an encoder $p_{\theta}(a | b)$ is a decoder. 
% We can derive a variational \textit{evidence lower bound} (ELBO) on $\log p_\theta(a)$, where $q_\phi(b | a)$ acts as an approximate posterior over $b \in \B$ as follows. For any $a \sim \pdata(a)$ and $b \sim \pdata(b)$ we can write:
% \begin{align}
% \log p_\theta(a) \nonumber \\
% =& \log p_\theta(a, b) - \log p_\theta(b | a) \\
% =& \log p_\theta(a | b) + \log p_\text{data}(b) - \log p_\theta(b | a)
% \intertext{We add and subtract the \textit{approximate posterior} $\log q_\phi(b | a)$}
% =& \log p_\theta(a | b) + \log p_\text{data}(b) - \log p_\theta(b | a) \nonumber \\
% & + \log q_\phi(b | a) - \log q_\phi(b | a) 
%  \intertext{By taking the expectation of both sides w.r.t $q_\phi(b | a)$ we get:}
% =&  \E_{b \sim q_\phi(b | a)} \big[ \log p_\theta(a | b) + \log p_\text{data}(b)  - \log q_\phi(b | a) \big] \nonumber \\
% &+ KL\big( q_\phi(b | a) \| p_\theta(b | a)\big) \\
% \geq& \E_{b \sim q_\phi(b | a)} \big[ \log p_\theta(a | b) \big]
%       - \E_{b \sim q_\phi(b | a)}\big[\log \frac{q_\phi(b | a)}{p_\text{data}(b)}  \big]
% \end{align}
% Hence, the ELBO is given by:
% \begin{align}
% \label{eq:elbo_cyclegan_a}
% \loss(a;&\theta, \phi) = \nonumber \\
% &\E_{b \sim q_\phi(b | a)} \big[ \log p_\theta(a | b) \big]
%      - \E_{b \sim q_\phi(b | a)}\big[\log \frac{q_\phi(b | a)}{p_\text{data}(b)}  \big]
% \end{align}
% The first term is a reconstruction loss term, which corresponds to forward cycle-consistency assuming that $p_\theta(a | b)$ follows a Laplace distribution with mean $G_\theta(F_\phi(a))$ and a fixed variance. The second term is a KL-divergence term that pushes $q_\phi(b | a)$ to be close to the prior $\pdata(b)$. Since $\pdata(b)$ is a complicated distribution which we have no explicit analytical for, minimizing the KL-divergence term can be \textit{approximated} using an adversarial approach introduced by~\citep{makhzani2015adversarial}, which is exactly what marginal matching in domain $\B$ achieves in CycleGAN.\footnote{Marginal matching in CycleGAN minimizes $KL(q_\phi(b)\|\pdata(b))$ instead of the proper $KL(q_\phi(b|a)\|\pdata(b))$. An alternative adversarial approach introduced by~\citep{mescheder2017adversarial} is shown to minimize the proper KL. It is obvious if in this context optimizing the proper KL would necessarily lead to better results, and we leave that for future work.} 
% Similarly, maximizing an ELBO over $\log q_\phi(b | a)$ for an autoencoder with $p_{\theta}(a | b)$ as an encoder and $q_\phi(b | a)$ as a decoder, corresponds to CycleGAN's backward cycle-consistency and marginal matching in $\A$. Combining these costs amounts to the full CycleGAN objective in Eqn.~\ref{eq:cgan_full_loss}. Therefore, we can see that CycleGAN is no more than two jointly-trained adversarial autoencoders.




% \subsection{Augmented CycleGAN as Two Adversarial Autoencoders with Auxiliary Variables}
% In this section we show that Augmented CycleGAN objective can be also derived using a variational framework, where autoencoders are equipped with auxiliary variables~\citep{maaloe2016auxiliary}.
% The forward and reverse mappings of Augmented CycleGAN  parameterize the following conditional distributions $q_\phi(b|a,z_b)$ and $p_{\theta}(a|b,z_a)$, respectively. The relationship between items in domains $\A$ and $\B$ is captured with the conditionals:
% \begin{eqnarray}
% p_{\theta}(a | b) &= & \int p_{\theta}(a | b, z_a)\pz(z_a) dz_a \\
% q_\phi(b | a) &= &  \int q_\phi(b | a, z_b)\pz(z_b) dz_b
% \end{eqnarray}
% These conditionals can fit more complicated relationships across domains than the ones defined by CycleGAN. 
% Using these conditionals, we can derive a similar ELBO for $\log p_\theta(a)$ as in Eqn.~\ref{eq:elbo_cyclegan_a}. The main difference here, however, is that conditionals include auxiliary variables $z_a$ and $z_b$ and cannot be directly optimized.  Nevertheless, we can rewrite the bound as follows:
% % \begin{eqnarray}
% % \loss(a;\theta, \phi) &=& \E_{b \sim q_\phi(b | a)} \big[ \log p_\theta(a | b) + \log p_\text{data}(b)  - \log q_\phi(b | a) \big]
% % %&=& \E_{b \sim q_\phi(b | a)} \big[ \log p_\theta(a | b) + \log p_\text{data}(b)\big] +  \E_{b \sim q_\phi(b | a)} \big[ - \log q_\phi(b | a) \big]  
% % \label{eq:elbo_aug_cgan}
% % \end{eqnarray}
% \begin{align}
% \label{eq:elbo_aug_cgan}
% \loss(a;&\theta, \phi) = \nonumber \\
% &\E_{b \sim q_\phi(b | a)} \big[ \log p_\theta(a | b)\big] +
% \E_{b \sim q_\phi(b | a)} \big[\log p_\text{data}(b) \big] +  \nonumber \\
% &\E_{b \sim q_\phi(b | a)}\big[-\log q_\phi(b | a)  \big]
% \end{align}
% The first term in corresponds to cycle-consistency but is intractable since conditionals include marginalization over latent variables. We derive a tractable lower bound for it in Sec.~\ref{sec:aug_cgan_cycle_elbo}.
% The final term, on the other hand, corresponds to the conditional entropy $H_{\phi}(b|a)$, which we can also derive a lower bound for as we show in Sec.~\ref{sec:aug_cgan_entropy_elbo}.
% In the following, we assume that encoders $E_\omega$ and $E_\gamma$ parameterize conditionals over latent variables $q_\omega(z_a|a,b)$ and $q_\gamma(z_b|a,b)$, respectively.

% \subsubsection{Deriving lower bound for cycle loss} \label{sec:aug_cgan_cycle_elbo}
% We derive a lower bound for $\log p_\theta(a | b)$, and then take its expected value with respect to $q_\phi(b | a)$ to get the full bound.
% \begin{align}
% \log &p_\theta(a | b) \nonumber \\ 
% &= \log p_\theta(a, z_a | b) - p_\theta(z_a | a, b) \nonumber \\
% &= \log p_\theta(a | z_a, b) + \log p_\theta(z_a | b) - \log p_\theta(z_a | a, b)
% \intertext{We assume that $z_a$ is marginally independent from $b$}
%      &= \log p_\theta(a | z_a, b) + \log p(z_a) - \log p_\theta(z_a | a, b) \\
%      \intertext{We define an \textit{approximate posterior} $q_\omega(z_a | a, b)$ over $z_a$, which we use to get the lower bound:}
%      &\geq \E_{z_a \sim q_\omega(z_a | a,b)} \big[ \log p_\theta(a | z_a, b)
%      - \log \frac{q_\omega(z_a | a,b)}{p(z_a)}  \big].
% \label{eq:cycle_elbo}
% \end{align}


% \subsubsection{Deriving lower bound for $H_{\phi}(b|a)$} \label{sec:aug_cgan_entropy_elbo}
% We can derive the lower bound on $H_{\phi}(b|a)$ by considering the conditional mutual information $I(b; z_b | a)$ between $b$ and $z_b$, given $a$ (eliding some $\phi$s):
% \begin{equation}
% I(b; z_b | a) = H(z_b | a) - H(z_b | a, b) = H(b | a) - H(b | a, z_b).
% \end{equation}
% We assume that $z_b$ and $a$ are marginally independent. We can rearrange terms to get the desired conditional entropy $H(b|a)$:
% \begin{equation}
% H(b|a) = H(z_b) - H(z_b|a,b) + H(b|a,z_b).
% \end{equation}

% % The first and last terms on the right (i.e.~$H(z_b|a)$ and $H(b|a,z_b)$) are equal to:
% % \begin{equation}
% % \E_{z_b \sim p(z_b)} \left[ \E_{b \sim q_\phi(b|a,z_b)} \left[ -\log q_\phi(z^a|a) -\log q_\phi(b|a, z^a) \right] \right]
% % \end{equation}
% % in Eqn.~\ref{eq:cond_ent_bound}. 
% We can drop the first term in the RHS since $\pz(z_b)$ has fixed entropy, and the last term since we assume $p(b|a,z_b)$ is a Laplace distribution with a fixed variance. 
% This leaves us with the (negative) conditional entropy $-H(z_b|a,b)$:
% \begin{equation}
% -H(z_b|a,b) = \E_{z_b \sim p(z_b)} \left[ \E_{b \sim q_\phi(b|a,z_b)} \left[ \log q_\phi(z_b|a,b) \right] \right],
% \end{equation}
% in which $q_\phi(z_b|a,b)$ denotes the true posterior over $z_b$ over $(b,z_b)$  defined by the forward mapping when conditioned on $a$, i.e. $q_\phi(b,z_b|a)=q_\phi(b|a,z_b)\pz(z_b)$. We can lower bound $-H_{\phi}(z_b|a,b)$ using an \textit{approximate inference} model $q_{\gamma}(z_b|a,b)$ parameterized by encoder $E_\gamma$:
% \begin{equation}
% -H_{\phi}(z_b|a,b) \geq \E_{z_b \sim p(z_b)} \left[ \E_{b \sim q_\phi(b|a,z_b)} \left[ \log q_\gamma(z_b|a,b) \right] \right].
% \label{eq:cond_ent_elbo}
% \end{equation}
% This bound is explained by non-negativity of the KL divergence:
% \begin{align}
% KL(&q_\phi(z_b|a,b) || q_\gamma(z_b|a,b)) = \nonumber \\
% &\E_{z_b \sim p(z_b)} \left[ \E_{b \sim q_\phi(b|a,z_b)} \left[ \log \frac{q_\phi(z_b|a,b)}{q_\gamma(z_b|a,b)} \right] \right]
% \end{align}
% for any distribution $q_\phi(z_b|a,b)$. I.e.:
% \begin{align}
% 0 \leq& \E_{z_b \sim p(z_b)} \left[ \E_{b \sim q_\phi(b|a,z_b)} \left[ \log \frac{q_\phi(z_b|a,b)}{q_\gamma(z_b|a,b)} \right] \right] \nonumber \\
% 0 \leq& \E_{z_b \sim \pz(z_b)} \left[ \E_{b \sim q_\phi(b|a,z_b)} \left[ \log q_\phi(z_b|a,b) - \log q_\gamma(z_b|a,b) \right] \right] \nonumber \\
% \;& \; \E_{z_b} \left[ \E_{b} \left[ \log q_\gamma(z_b|a,b) \right] \right] \leq \E_{z_b} \left[ \E_{b} \left[ \log q_\phi(z_b|a,b) \right] \right]
% \end{align}


% \subsubsection{Full bound for Augmented CycleGAN model}
% We can now use the bounds in Eqn.~\ref{eq:cycle_elbo} and Eqn.~\ref{eq:cond_ent_elbo} to rewrite a full bound for the model in Eqn.~\ref{eq:elbo_aug_cgan}:
% \begin{align}
% \label{eq:final_elbo_aug_cgan}
% \loss&(a;\theta, \phi) \nonumber \\ 
% = &\E_{b \sim q_\phi(b | a)} \big[ \log p_\theta(a | b)\big] + \E_{b \sim q_\phi(b | a)} \big[\log p_\text{data}(b) \big] +  \nonumber \\
% &\E_{b \sim q_\phi(b | a)}\big[-\log q_\phi(b | a)  \big] \nonumber \\
% \geq &\E_{z_b \sim p(z_b)} 
%  \Bigg[ \E_{b \sim q_\phi(b|a,z_b)} \bigg[ \log q_\gamma(z_b|a,b)- \log \frac{q_\phi(b|a, z_b)}{p_\text{data}(b)} + \nonumber \\
% &\,\,\,\,\,\,\,\,\,\,\,\, 
% \E_{z_a \sim q_\omega(z_a|a,b)} \big[ \log p_\theta(a|z_a,b) - \log \frac{q_\omega(z_a|a,b)}{p(z_a)} \big] \bigg] \Bigg]
% \end{align}

% For any $a \in \A$, $b \in \B$ and $z_a \in \Za$ we can write:
% \begin{align}
% \log p_\theta(a) \nonumber \\
% =& \log p_\theta(a, b, z_a) - \log p_\theta(b, z_a | a) \\
% =& \log p_\theta(a | b, z_a) + \log p_\text{data}(b) - \log \pz(z_a) \nonumber \\
% & - \log p_\theta(b, z_a | a)
% \intertext{We add and subtract the \textit{approximate posterior} $\log q_\phi(b, z_a | a)$}
% =& \log p_\theta(a | b, z_a) + \log p_\text{data}(b) - \log \pz(z_a) \nonumber \\
% & - \log p_\theta(b, z_a | a) + \log q_\phi(b, z_a | a) - \log q_\phi(b, z_a | a)
%  \intertext{We take the expectation of both sides w.r.t $q_\phi(b, z_a | a)$}
% =&  \E_{b, z_a \sim q_\phi(b | a)} \big[ \log p_\theta(a | b) + \log p_\text{data}(b)  - \log q_\phi(b | a) \big] \nonumber \\
% &+ KL\big( q_\phi(b | a) \| p_\theta(b | a)\big) \\
% \geq& \E_{b \sim q_\phi(b | a)} \big[ \log p_\theta(a | b) \big]
%       - \E_{b \sim q_\phi(b | a)}\big[\log \frac{q_\phi(b | a)}{p_\text{data}(b)}  \big]     
% \end{align}

% \subsubsection{Entropy considerations}

% Consider two domains $\mathcal{A}$, $\mathcal{B}$. Assume that we have two random samples $\{a_i\}_{i=1}^n$ and $\{b_j\}_{j=1}^m$ drawn from unknown probability distributions $p_A$, $p_B$ defined on $\mathcal{A}$ and $\mathcal{B}$ respectively. Assume a mapping $f_{AB}: \mathcal{A} \rightarrow \mathcal{B}$, $b^\prime = f_{AB}(a)$. Consider a similar mapping $f_{BA}: \mathcal{B} \rightarrow \mathcal{A}$, $a^\prime = f_{BA}(b)$. $b^\prime$ is a random variable following an unknown distribution $b^\prime \sim q_B$ (if the mapping $f$ is smooth and invertible we can say something about $q$). However, we can say that $H(q_B) \leq H(p_A)$, where inequality is obtained if $f$ is contractive.

% By adding the \emph{marginal matching} cost, which restrict $q_B$ to look like $p_B$, we have an additional constraint that $H(q_B) \leq \min \{H(p_A), H(q_B)\}$. 

% Let's introduce the \emph{cycle consistency} cost as $C = d(a, f_{BA}(f_{AB}(a))$, where $d$ is a divergence measure for which $\min d = 0$. A necessary condition for the solution $f_{AB}^* = \arg\min_{f_{AB}} C$ is that $H(q^*_B) \geq H(p_A)$ [PROVE], where $q^*_B$ is the distribution induced on $\mathcal{B}$ by the optimal mapping $f_{AB}^*$. However, because of the restriction on the class of mappings $f_{AB}$, the only viable solution for $f_{AB}^*$ is such that $H(q^*_B) = H(p_A)$.

% Now, let's switch to the case in which $f^{AB}$, $f^{BA}$ are stochastic mappings, i.e. $\tilde f^{AB}$ is a deterministic mapping from an extended space $\tilde f^{AB}: \mathcal{A} \times \mathcal{Z} \rightarrow \mathcal{B}$, and $f^{AB}$. When learning stochastic mappings from between domains, a desirable property would be that 

\subsection{Experimental Details} \label{sec:experiment_details}

\subsubsection{Edges-to-Shoes} \label{sec:e2s_exp_details}
In this section we describe in detail the architecture and training details for edges to shoes experiment. The dataset is the same used in \cite{isola2017image}. Specifically we shuffle the data such that it is no more paired. The networks architectural details for generators, discriminators and encoder are as described in table\ref{tab:shoes_arch_description}. For optimization we used Adam \cite{KingmaB14} as optimizer with learning rate 0.001 for generator and discriminator networks. For conditioning the latent code in the generator, Conditional Instance Norm \cite{dumoulin2016learned} is used. We trained the Augmented-CycleGAN for 200,000 iterations with batch-size of 50 to achieve the desired results.
\subsubsection{Male-to-Female} \label{sec:m2f_exp_details}
Here we state the experimental details of Male to Female mappings on high resolution($128 \times 128$)CelebA dataset\cite{liu2015faceattributes}. The network architectures are summarized in table \ref{tab:m2f_arch_description}.  For generator we also experimented with the unet architecture similar to the one used in \cite{zhu2017toward}. Hyper-parameters are same as mentioned in the previous section for edges-to-shoes \\
% \begin{enumerate}
%     \item \textbf{Generator:} 

% {\fontfamily{qcr}\selectfont 

% INPUT(64*64*3)-C(3,64;7c1s)-CIN-ReLU-C(64,128;3c1s)-CIN-ReLU-C(128,256;3c2s)-CIN-ReLU-3*[ResnetBlock(256;3c1s)-CIN-ReLU]-DC(256,128;4c2s)-CIN-ReLU-[ResnetBlock(128;3c1s)-CIN-ReLU]-C(128,64;3c1s)-CIN-ReLU-C(64,3;3c1s)-Tanh-OUTPUT(64*64*3)



% } 
% \end{enumerate}
% Note that C(3,64;7c1s) refers a convolutional layer with 3-input channels, 64 output channels kernel size of 7 and stride 1, DC stands for Deconvolutional layer. CIN referes to Conditional Instance Normalization and ReLU, Tanh are the activation functions used.


% \subsubsection{Attributes-to-Faces} \label{sec:a2f_exp_details}
% In this section we describe the experimnetal details and architectural considerations for attributes to faces experiment. For fair comparision, our generator from attributes to faces is the same as that of \cite{gan2017triangle}
% \begin{table*}[t!]
% \centering
% \begin{tabular}{@{}rllllll@{}} 
% Operation              & Kernel       & Strides      & Feature maps & CIN/IN/BN?      & Dropout & Nonlinearity \\ \midrule
% $G_{A-B}(x)$ -- $3 \times 64 \times 64$ input                                                             \\
% Reflection Pading(3) \\
% Convolution            & $7 \times 7$ & $1 \times 1$ & $64$         & CIN  & 0.0     & Leaky ReLU \\
% Convolution            & $3 \times 3$ & $1 \times 1$ & $128$         & CIN  & 0.0     & Leaky ReLU \\
% Convolution            & $3 \times 3$ & $2 \times 2$ & $256$         & CIN  & 0.0     & Leaky ReLU \\
% CINResnet Block           & $3 \times 3$ & $1 \times 1$ & $256$        & CIN  & 0.0     & Leaky ReLU \\
% CINResnet Block           & $3 \times 3$ & $1 \times 1$ & $256$        & CIN  & 0.0     & Leaky ReLU \\
% CINResnet Block           & $3 \times 3$ & $1 \times 1$ & $256$        & CIN  & 0.0     & Leaky ReLU \\
% CINResnet Block           & $3 \times 3$ & $1 \times 1$ & $256$        & CIN  & 0.0     & Leaky ReLU \\
% TransposeConv            & $3 \times 3$ & $2 \times 2$ & $128$        & CIN & 0.0     & Leaky ReLU \\
% CINResnet Block           & $3 \times 3$ & $1 \times 1$ & $128$        & CIN  & 0.0     & Leaky ReLU \\
% Convolution            & $3 \times 3$ & $1 \times 1$ & $64$        & CIN & 0.0     & Leaky ReLU     \\
% Convolution            & $3 \times 3$ & $1 \times 1$ & $3$        & $\times$ & 0.0     & Tanh     
% %  Gaussian Layer \\
% % $G_{z_2}(z_1)$ -- $64 \times 32 \times 32$ input                                                              \\
% % Convolution            & $3 \times 3$ & $2 \times 2$ & $256$         & BN  & 0.0     & Leaky ReLU \\
% % Convolution            & $3 \times 3$ & $2 \times 2$ & $256$         & BN  & 0.0     & Leaky ReLU \\
% % % $Resnet Block$           & $3 \times 3$ & $2 \times 2$ & $64$        & $\surd$  & 0.0     & Leaky ReLU \\
% % Convolution           & $3 \times 3$ & $2 \times 2$ & $512$        & BN  & 0.0     & Leaky ReLU \\
% % Resnet Block            & $3 \times 3$ & $1 \times 1$ & $512$        & BN  & 0.0     & Leaky ReLU \\
% % Convolution             & $4 \times 4$ & $valid$ & $512$        & BN  & 0.0     & Leaky ReLU \\
% % Convolution            & $1 \times 1$ & $1 \times 1$ & $512$        & $\times$ & 0.0     & Linear     
% \\ \midrule
% $G_{B-A}(x)$ -- $3 \times 64 \times 64$ input                                                             \\
% Reflection Pading(3) \\
% Convolution            & $7 \times 7$ & $1 \times 1$ & $64$         & IN  & 0.0     & Leaky ReLU \\
% Convolution            & $3 \times 3$ & $1 \times 1$ & $128$         & IN  & 0.0     & Leaky ReLU \\
% Convolution            & $3 \times 3$ & $2 \times 2$ & $256$         & IN  & 0.0     & Leaky ReLU \\
% Resnet Block           & $3 \times 3$ & $1 \times 1$ & $256$        & IN  & 0.0     & Leaky ReLU \\
% Resnet Block           & $3 \times 3$ & $1 \times 1$ & $256$        & IN  & 0.0     & Leaky ReLU \\
% Resnet Block           & $3 \times 3$ & $1 \times 1$ & $256$        & IN  & 0.0     & Leaky ReLU \\
% Resnet Block           & $3 \times 3$ & $1 \times 1$ & $256$        & IN  & 0.0     & Leaky ReLU \\
% TransposeConv            & $3 \times 3$ & $2 \times 2$ & $128$        & IN & 0.0     & Leaky ReLU \\
% Resnet Block           & $3 \times 3$ & $1 \times 1$ & $128$        & IN  & 0.0     & Leaky ReLU \\
% Convolution            & $3 \times 3$ & $1 \times 1$ & $64$        & IN & 0.0     & Leaky ReLU     \\
% Convolution            & $3 \times 3$ & $1 \times 1$ & $3$        & $\times$ & 0.0     & Tanh     
% \\ \midrule
% $E_{B}(x)$ -- $3 \times 64 \times 64$ input                                                             \\

% Convolution            & $3 \times 3$ & $2 \times 2$ & $64$         & BN  & 0.0     & Leaky ReLU \\
% Convolution            & $3 \times 3$ & $2 \times 2$ & $128$         & BN  & 0.0     & Leaky ReLU \\
% Convolution            & $3 \times 3$ & $2 \times 2$ & $256$         & BN  & 0.0     & Leaky ReLU \\

% Convolution            & $3 \times 3$ & $2 \times 2$ & $512$        & BN & 0.0     & Leaky ReLU     \\
% Convolution            & $4 \times 4$ & $valid$ & $512$        & $\times$ & 0.0     & Leaky ReLU\\    
% Convolution            & $1 \times 1$ & $valid$ & $2*nlatent$        & $\times$ & 0.0     & None    
% \\ \midrule
% $D_B(x)$ -- $3 \times 64 \times 64$ input                                                               \\
% Convolution            & $3 \times 3$ & $2 \times 2$ & $64$         & BN  & 0.0     & Leaky ReLU \\
% Convolution            & $3 \times 3$ & $2 \times 2$ & $128$         & BN  & 0.0     & Leaky ReLU \\
% Convolution            & $3 \times 3$ & $1 \times 1$ & $256$         & BN  & 0.0     & Leaky ReLU \\

% Convolution            & $3 \times 3$ & $1 \times 1$ & $512$        & BN & 0.0     & Leaky ReLU     \\
% Convolution            & $3 \times 3$ & $valid$ & $1$        & $\times$ & 0.0     & None    
    
% \\ \midrule

% $D_A(x)$ -- $3 \times 64 \times 64$ input                                                               \\
% Convolution            & $3 \times 3$ & $2 \times 2$ & $64$         & BN  & 0.0     & Leaky ReLU \\
% Convolution            & $3 \times 3$ & $2 \times 2$ & $128$         & BN  & 0.0     & Leaky ReLU \\
% Convolution            & $3 \times 3$ & $1 \times 1$ & $256$         & BN  & 0.0     & Leaky ReLU \\

% Convolution            & $3 \times 3$ & $1 \times 1$ & $512$        & BN & 0.0     & Leaky ReLU     \\
% Convolution            & $3 \times 3$ & $valid$ & $1$        & $\times$ & 0.0     & None    \\     \midrule
% %Optimizer              & \multicolumn{6}{@{}l@{}}{Adam ($\alpha = 10^{-4}$, $\beta_1 = 0.5$, $\beta_2 = 10^{-3}$)} \\
% %Batch size             & \multicolumn{6}{@{}l@{}}{128}												  \\
% %Epochs                 & \multicolumn{6}{@{}l@{}}{100}  											  \\
% %Leaky ReLU slope       & \multicolumn{6}{@{}l@{}}{0.1}                                                \\
% %Weight, bias initialization  & \multicolumn{6}{@{}l@{}}{Isotropic gaussian ($\mu = 0$, $\sigma = 0.01$), Constant($0$)} \\ \bottomrule
% \end{tabular}
% \vspace{0.2cm} 
% \caption{\label{tab:shoes_arch_description} Architecture detail for AugmentedCycleGAN(unsupervised) on the Edges-to-shoes  Datasets.}

% \end{table*}


% \begin{table*}[t!]
% \centering
% \begin{tabular}{@{}rllllll@{}} 
% Operation              & Kernel       & Strides      & Feature maps & CIN/IN/BN?      & Dropout & Nonlinearity \\ \midrule
% $G_{A-B}(x)$ -- $3 \times 128 \times 128$ input                                                             \\
% Reflection Pading(3) \\
% Convolution            & $7 \times 7$ & $1 \times 1$ & $64$         & CIN  & 0.0     & Leaky ReLU \\
% Convolution            & $3 \times 3$ & $1 \times 1$ & $128$         & CIN  & 0.0     & Leaky ReLU \\
% Convolution            & $3 \times 3$ & $2 \times 2$ & $256$         & CIN  & 0.0     & Leaky ReLU \\
% CINResnet Block           & $3 \times 3$ & $1 \times 1$ & $256$        & CIN  & 0.0     & Leaky ReLU \\
% CINResnet Block           & $3 \times 3$ & $1 \times 1$ & $256$        & CIN  & 0.0     & Leaky ReLU \\
% CINResnet Block           & $3 \times 3$ & $1 \times 1$ & $256$        & CIN  & 0.0     & Leaky ReLU \\
% CINResnet Block           & $3 \times 3$ & $1 \times 1$ & $256$        & CIN  & 0.0     & Leaky ReLU \\
% TransposeConv            & $3 \times 3$ & $2 \times 2$ & $128$        & CIN & 0.0     & Leaky ReLU \\
% CINResnet Block           & $3 \times 3$ & $1 \times 1$ & $128$        & CIN  & 0.0     & Leaky ReLU \\
% Convolution            & $3 \times 3$ & $1 \times 1$ & $64$        & CIN & 0.0     & Leaky ReLU     \\
% Convolution            & $3 \times 3$ & $1 \times 1$ & $3$        & $\times$ & 0.0     & Tanh     
% %  Gaussian Layer \\
% % $G_{z_2}(z_1)$ -- $64 \times 32 \times 32$ input                                                              \\
% % Convolution            & $3 \times 3$ & $2 \times 2$ & $256$         & BN  & 0.0     & Leaky ReLU \\
% % Convolution            & $3 \times 3$ & $2 \times 2$ & $256$         & BN  & 0.0     & Leaky ReLU \\
% % % $Resnet Block$           & $3 \times 3$ & $2 \times 2$ & $64$        & $\surd$  & 0.0     & Leaky ReLU \\
% % Convolution           & $3 \times 3$ & $2 \times 2$ & $512$        & BN  & 0.0     & Leaky ReLU \\
% % Resnet Block            & $3 \times 3$ & $1 \times 1$ & $512$        & BN  & 0.0     & Leaky ReLU \\
% % Convolution             & $4 \times 4$ & $valid$ & $512$        & BN  & 0.0     & Leaky ReLU \\
% % Convolution            & $1 \times 1$ & $1 \times 1$ & $512$        & $\times$ & 0.0     & Linear     
% \\ \midrule
% $G_{B-A}(x)$ -- $3 \times 64 \times 64$ input                                                             \\
% Reflection Pading(3) \\
% Convolution            & $7 \times 7$ & $1 \times 1$ & $64$         & CIN  & 0.0     & Leaky ReLU \\
% Convolution            & $3 \times 3$ & $1 \times 1$ & $128$         & CIN  & 0.0     & Leaky ReLU \\
% Convolution            & $3 \times 3$ & $2 \times 2$ & $256$         & CIN  & 0.0     & Leaky ReLU \\
% CINResnet Block           & $3 \times 3$ & $1 \times 1$ & $256$        & CIN  & 0.0     & Leaky ReLU \\
% CINResnet Block           & $3 \times 3$ & $1 \times 1$ & $256$        & CIN  & 0.0     & Leaky ReLU \\
% CINResnet Block           & $3 \times 3$ & $1 \times 1$ & $256$        & CIN  & 0.0     & Leaky ReLU \\
% CINResnet Block           & $3 \times 3$ & $1 \times 1$ & $256$        & CIN  & 0.0     & Leaky ReLU \\
% TransposeConv            & $3 \times 3$ & $2 \times 2$ & $128$        & CIN & 0.0     & Leaky ReLU \\
% CINResnet Block           & $3 \times 3$ & $1 \times 1$ & $128$        & CIN  & 0.0     & Leaky ReLU \\
% Convolution            & $3 \times 3$ & $1 \times 1$ & $64$        & CIN & 0.0     & Leaky ReLU     \\
% Convolution            & $3 \times 3$ & $1 \times 1$ & $3$        & $\times$ & 0.0     & Tanh   
% \\ \midrule
% $E_{B}(x)$ -- $3 \times 128 \times 128$ input                                                             \\

% Convolution            & $3 \times 3$ & $2 \times 2$ & $64$         & BN  & 0.0     & Leaky ReLU \\
% Convolution            & $3 \times 3$ & $2 \times 2$ & $128$         & BN  & 0.0     & Leaky ReLU \\
% Convolution            & $3 \times 3$ & $2 \times 2$ & $256$         & BN  & 0.0     & Leaky ReLU \\

% Convolution            & $3 \times 3$ & $2 \times 2$ & $512$        & BN & 0.0     & Leaky ReLU     \\
% Convolution            & $3 \times 3$ & $2 \times 2$ & $512$        & BN & 0.0     & Leaky ReLU     \\
% Convolution            & $4 \times 4$ & $valid$ & $512$        & $\times$ & 0.0     & Leaky ReLU\\    
% Convolution            & $1 \times 1$ & $valid$ & $2*nlatent$        & $\times$ & 0.0     & None    
% \\ \midrule
% $D_B(x)$ -- $3 \times 128 \times 128$ input                                                               \\
% Convolution            & $3 \times 3$ & $2 \times 2$ & $64$         & BN  & 0.0     & Leaky ReLU \\
% Convolution            & $3 \times 3$ & $2 \times 2$ & $128$         & BN  & 0.0     & Leaky ReLU \\
% Convolution            & $3 \times 3$ & $2 \times 2$ & $128$         & BN  & 0.0     & Leaky ReLU \\
% Convolution            & $3 \times 3$ & $1 \times 1$ & $256$         & BN  & 0.0     & Leaky ReLU \\

% Convolution            & $3 \times 3$ & $1 \times 1$ & $512$        & BN & 0.0     & Leaky ReLU     \\
% Convolution            & $3 \times 3$ & $valid$ & $1$        & $\times$ & 0.0     & None    
    
% \\ \midrule

% $D_A(x)$ -- $3 \times 128 \times 128$ input                                                               \\
% Convolution            & $3 \times 3$ & $2 \times 2$ & $64$         & BN  & 0.0     & Leaky ReLU \\
% Convolution            & $3 \times 3$ & $2 \times 2$ & $128$         & BN  & 0.0     & Leaky ReLU \\
% Convolution            & $3 \times 3$ & $2 \times 2$ & $128$         & BN  & 0.0     & Leaky ReLU \\
% Convolution            & $3 \times 3$ & $1 \times 1$ & $256$         & BN  & 0.0     & Leaky ReLU \\

% Convolution            & $3 \times 3$ & $1 \times 1$ & $512$        & BN & 0.0     & Leaky ReLU     \\
% Convolution            & $3 \times 3$ & $1 \times 1$ & $1$        & $\times$ & 0.0     & None\\     \midrule
% %Optimizer              & \multicolumn{6}{@{}l@{}}{Adam ($\alpha = 10^{-4}$, $\beta_1 = 0.5$, $\beta_2 = 10^{-3}$)} \\
% %Batch size             & \multicolumn{6}{@{}l@{}}{128}												  \\
% %Epochs                 & \multicolumn{6}{@{}l@{}}{100}  											  \\
% %Leaky ReLU slope       & \multicolumn{6}{@{}l@{}}{0.1}                                                \\
% %Weight, bias initialization  & \multicolumn{6}{@{}l@{}}{Isotropic gaussian ($\mu = 0$, $\sigma = 0.01$), Constant($0$)} \\ \bottomrule
% \end{tabular}
% \vspace{0.2cm} 
% \caption{\label{tab:m2f_arch_description} Architecture detail for AugmentedCycleGAN(unsupervised) on the Male-to-Female Datasets.}

% \end{table*}
% \begin{table*}
% \centering
% \begin{tabular}{l|l|l|}

% \hline
% \textbf{Generator A to B}&\textbf{Generator B to A}& \textbf{Discriminator}\\% \Tstrut\Bstrut\\

% \hline
%   \makecell{Layer}   & \makecell{number of outputs \\} &  kernel size &stride&activation function\\% \Tstrut\Bstrut\\ 
% \hlx{vhv}


%  input $x \sim p_{data}$ or $\mathcal{G}$ & $28 \times 28 \times 3$ & \\


% convolution & 14*14*64 & $5\times 5\\
%  convolution & 7*7*128 & $5\times 5\\
%  convolution& 4*4*256 & $5\times 5\\
% convolution& 2*2*512 & $5\times 5\\
% fully-connected& 1 & \\
% \hline
% \end{tabular}
% \caption{ network for attributes to faces experiment}
% \label{table:attributes2faces_arc}
% \end{table*}
